# Supplementary material for: On a Heegaard Floer theory for tangles
Source: arXiv:1610.07494 ancillary file (2017-03-07)
Supplement: Supplementary file 1 [file 0.HDs.pdf]

Nice Heegaard diagram for  $2m_3pt$  BSD.nb

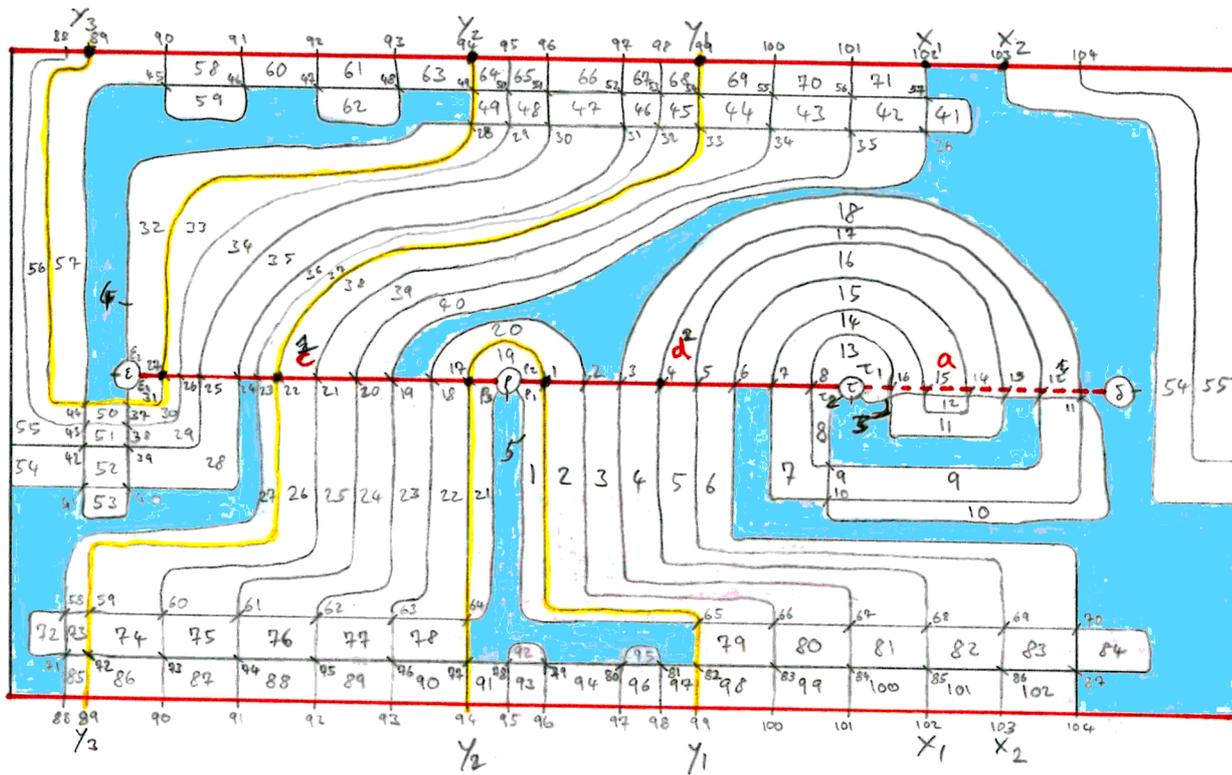

Arc diagram for  $2m_3pt$  BSD.nb

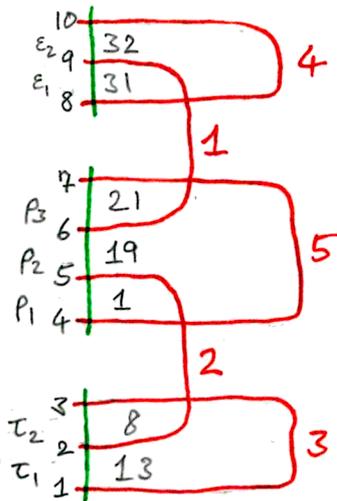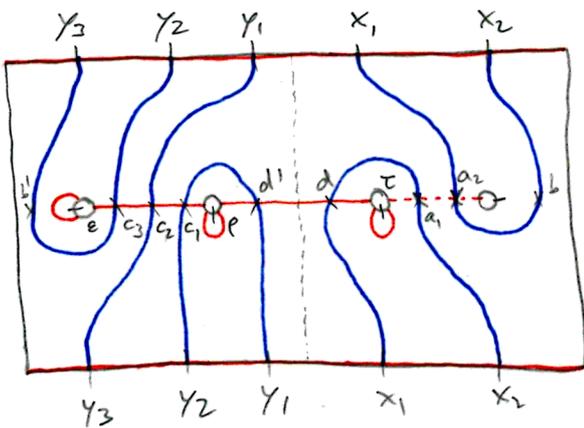

Arc diagram for  $2m_3pt$  met BSD.nb

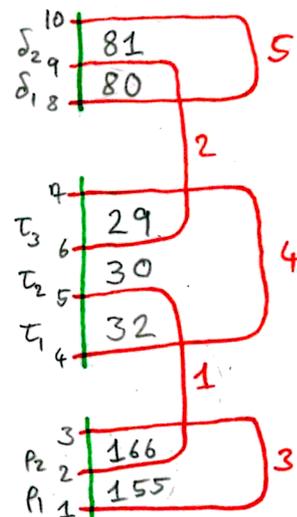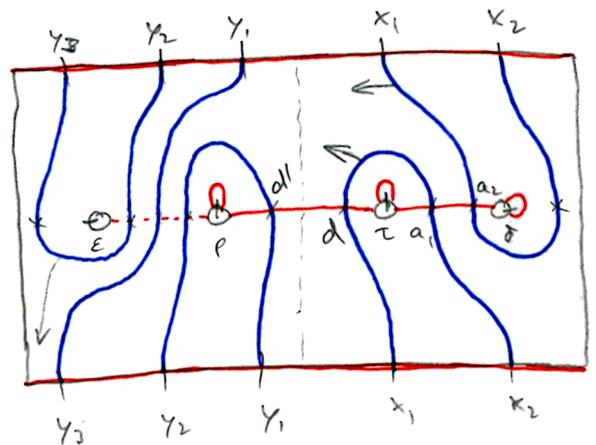

Nice HD for ZmSptmt BSD.u6

NR=221 NI=223

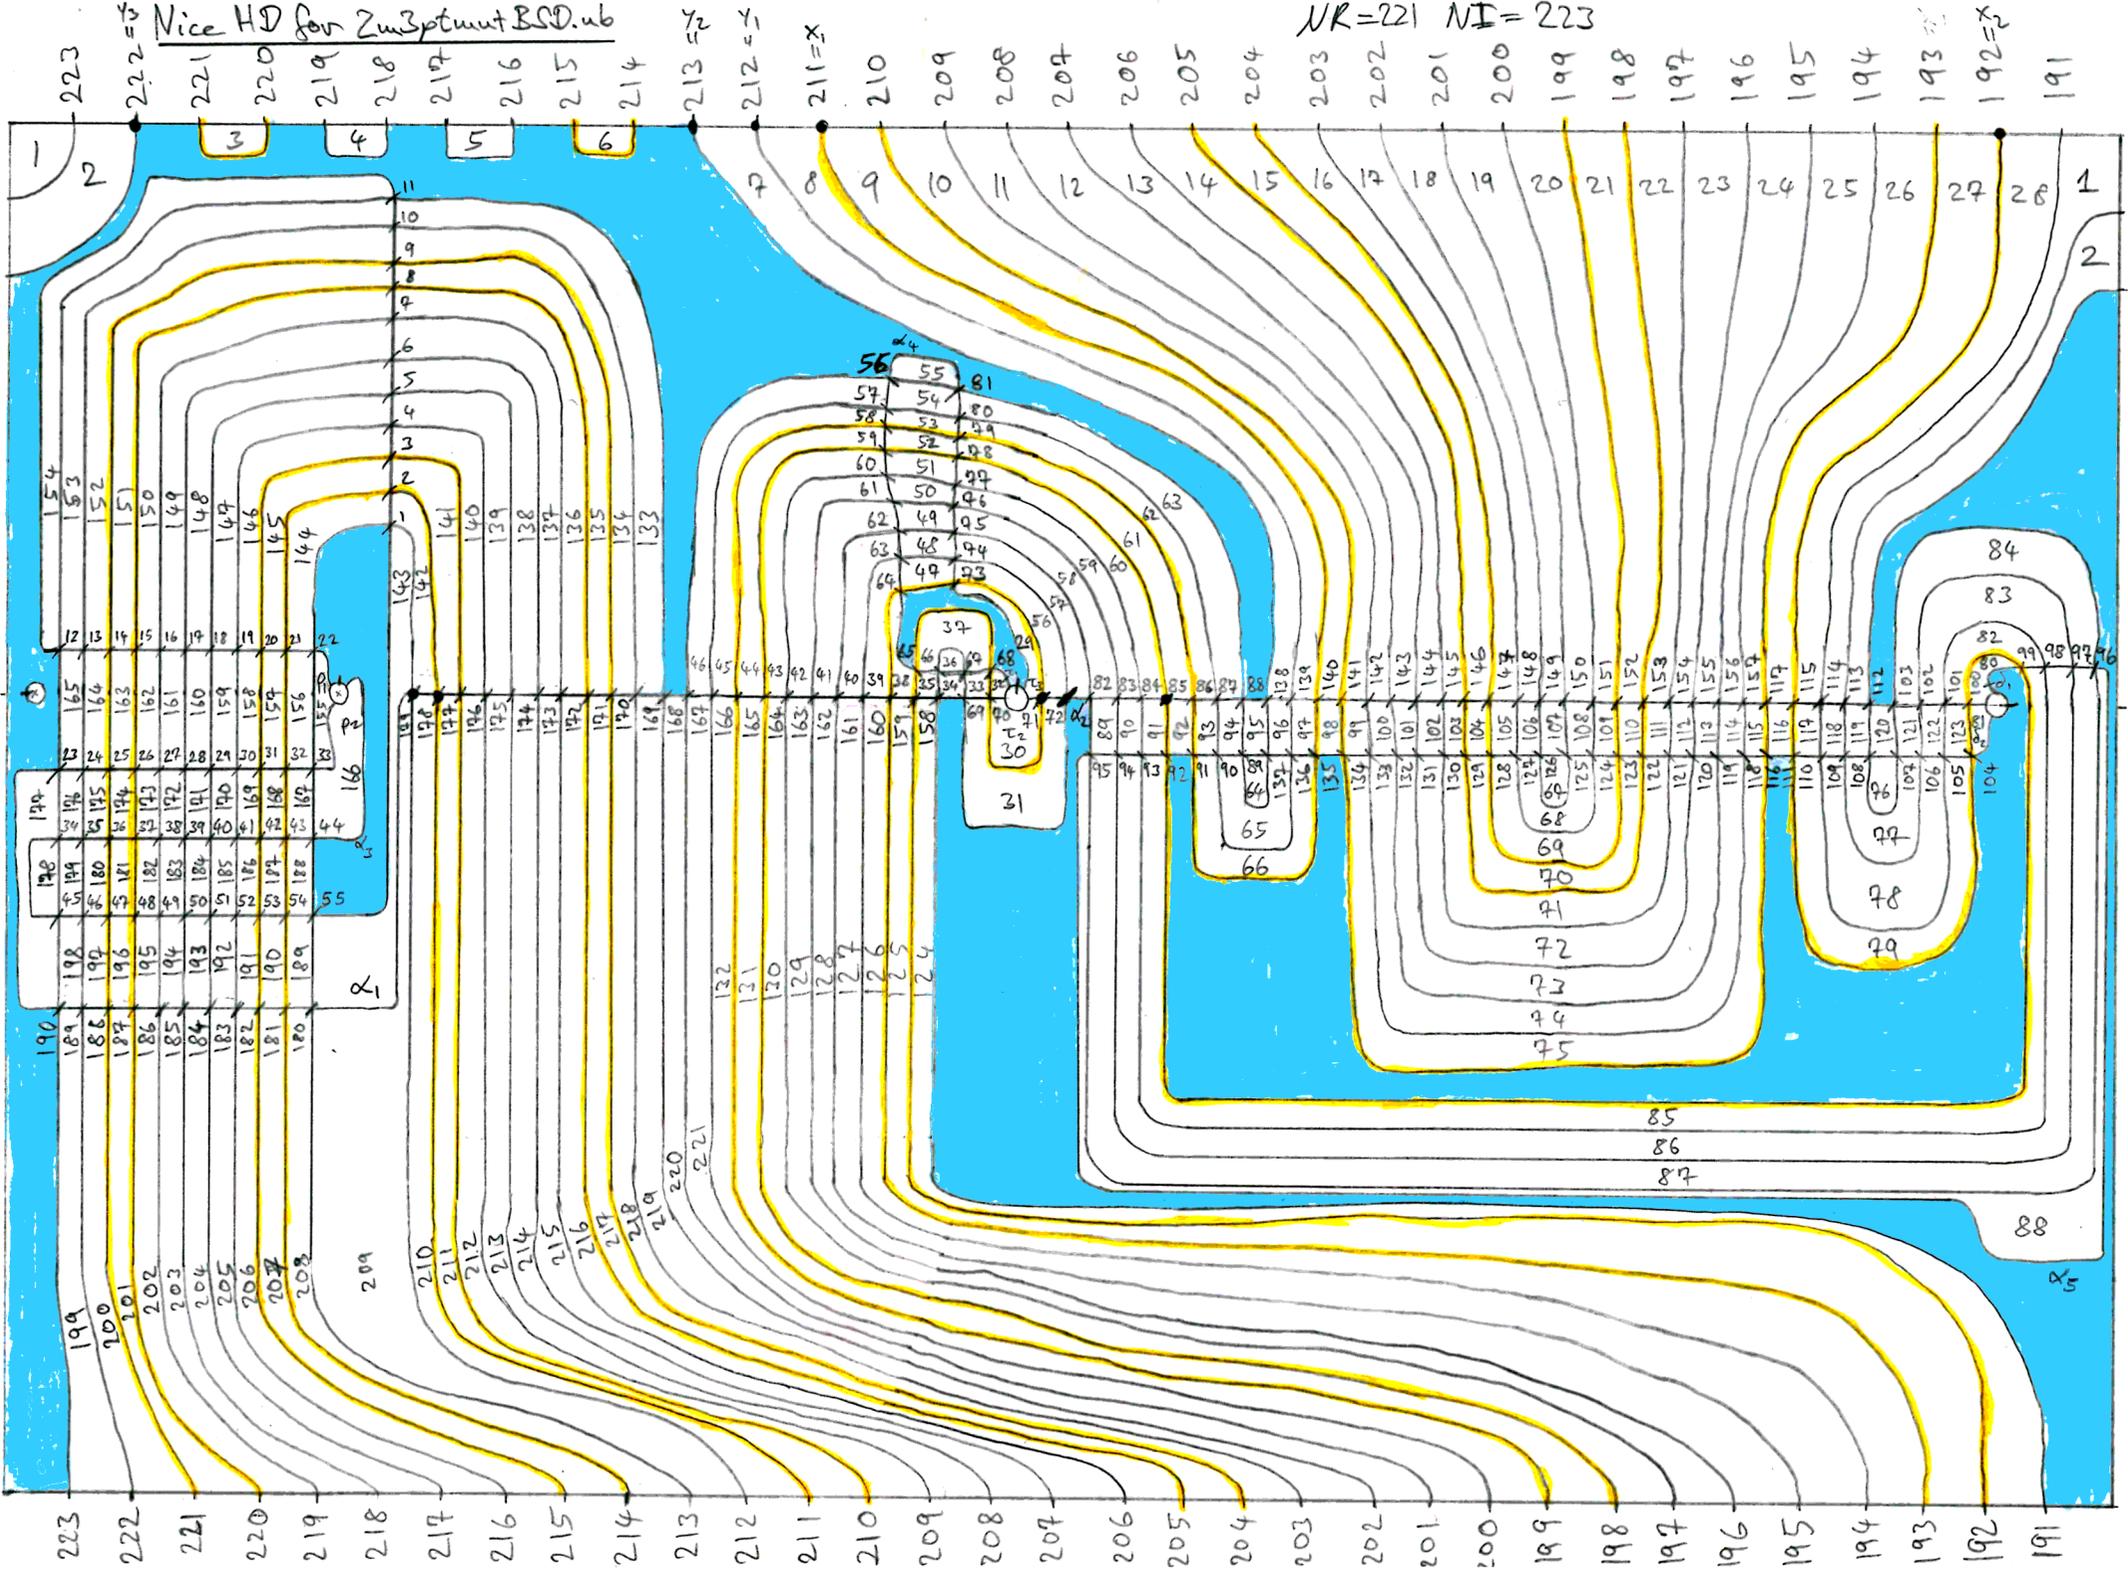

Glueing  $BSAA \times 4e$ .ub

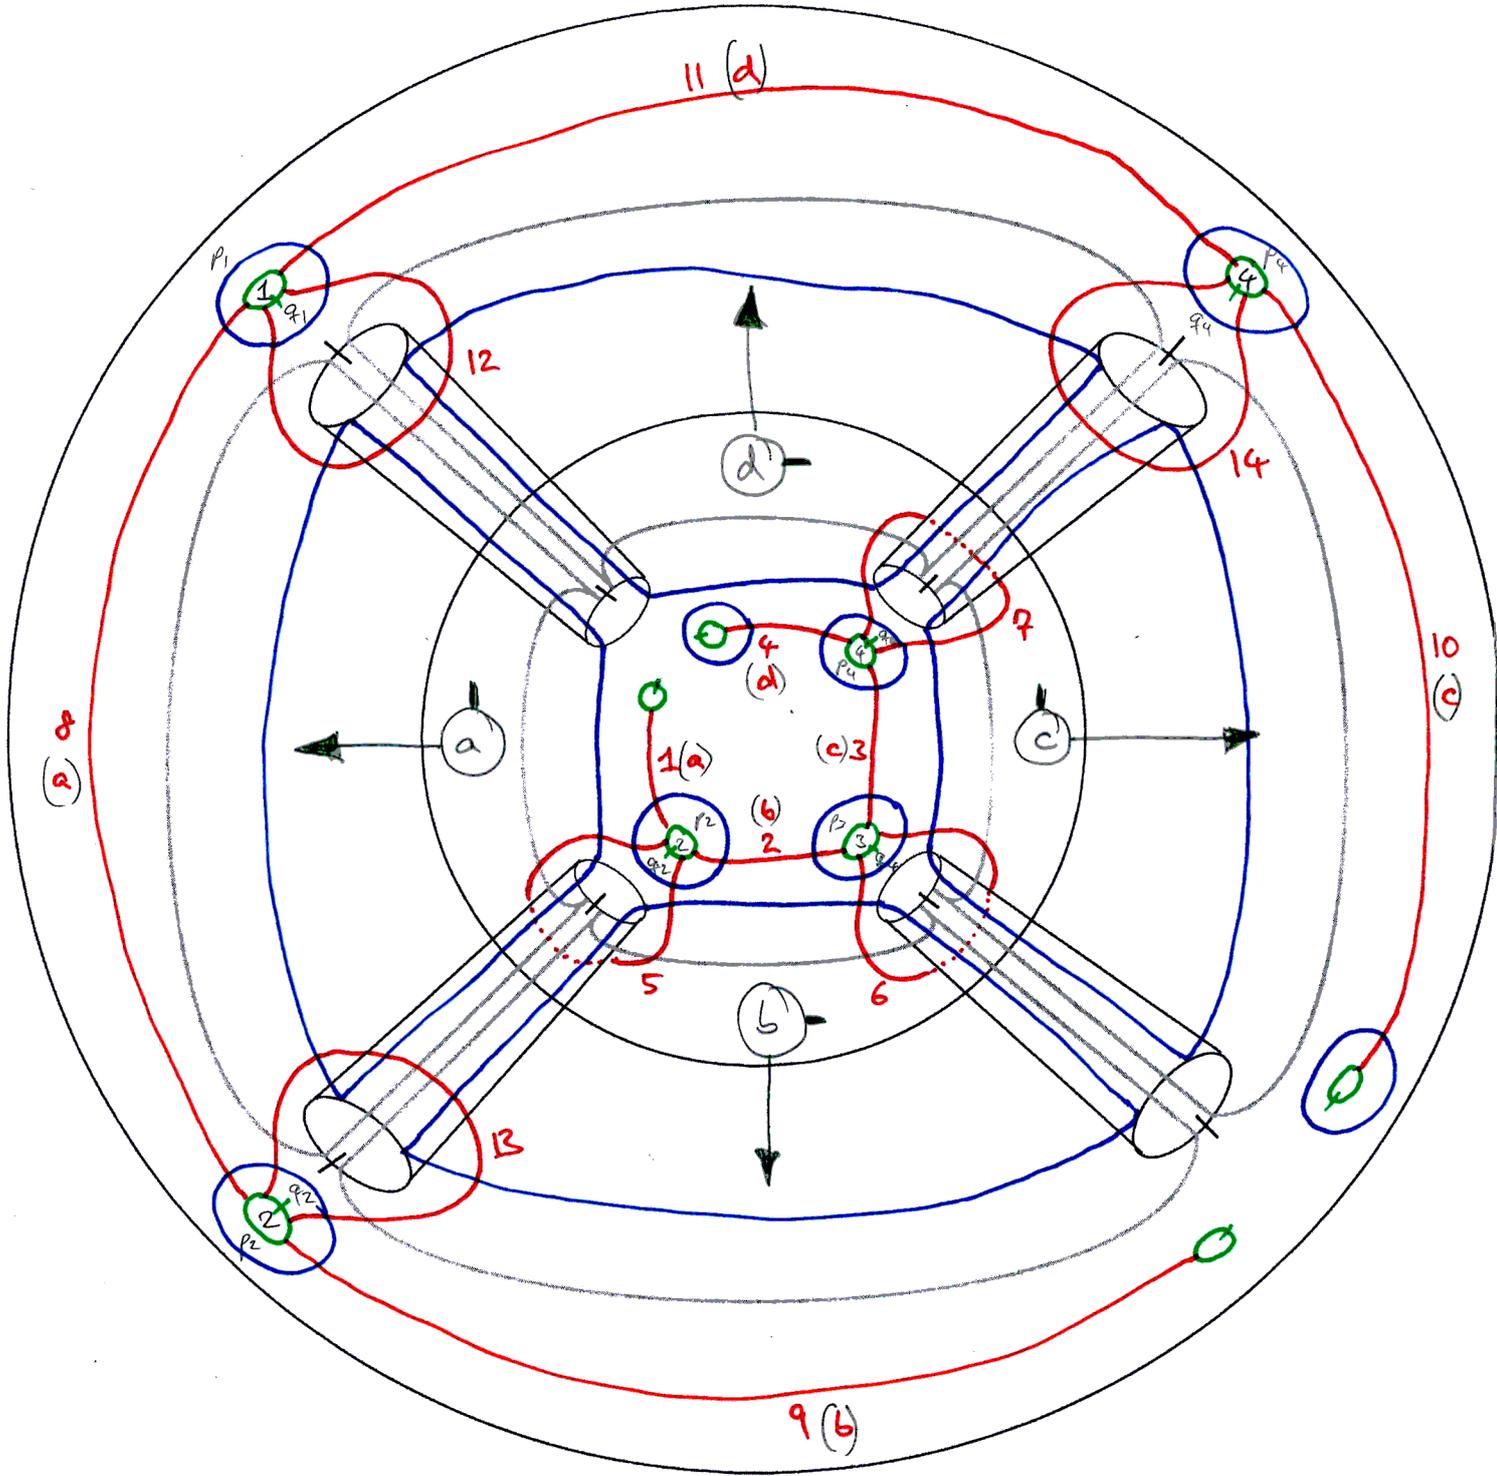

outer  
inner

Back

Glueing  $[BSAA \times 4e]_{ub}$

Front

inner  
outer

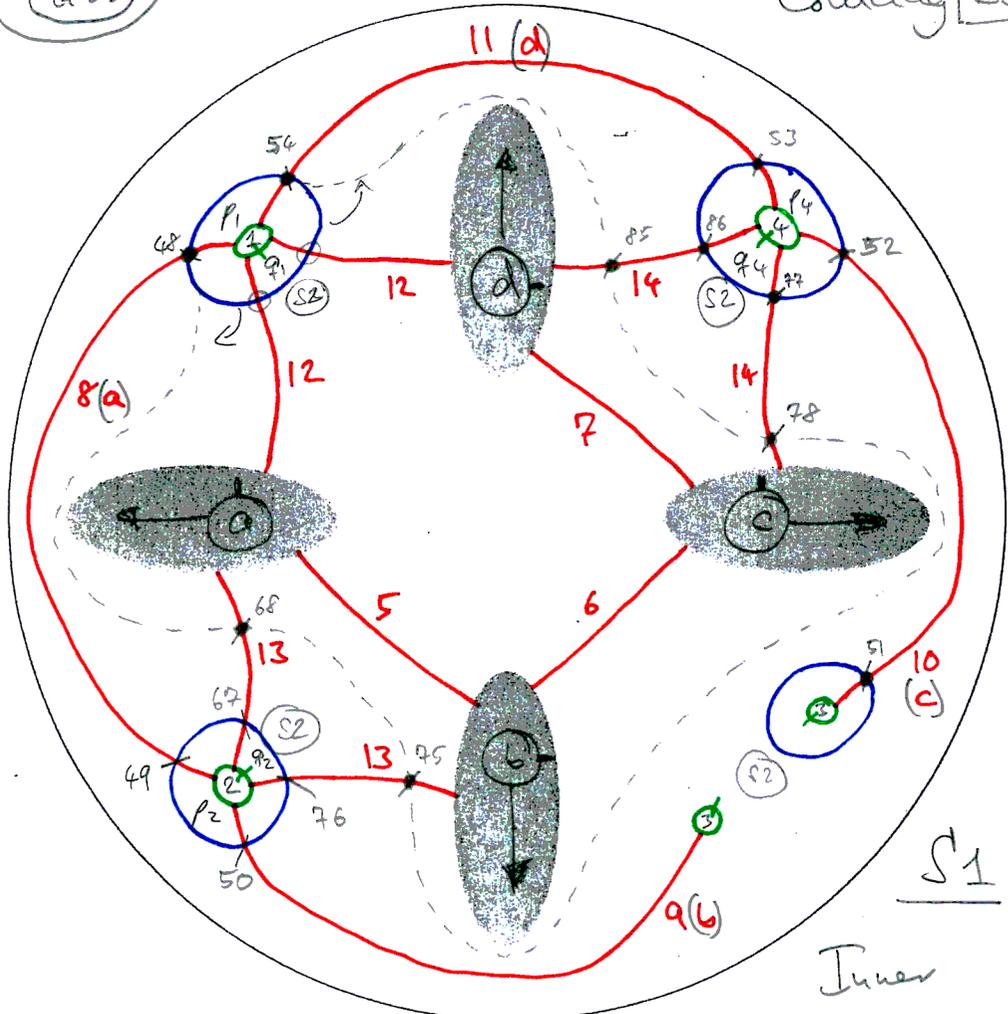

$S_1$

Inner

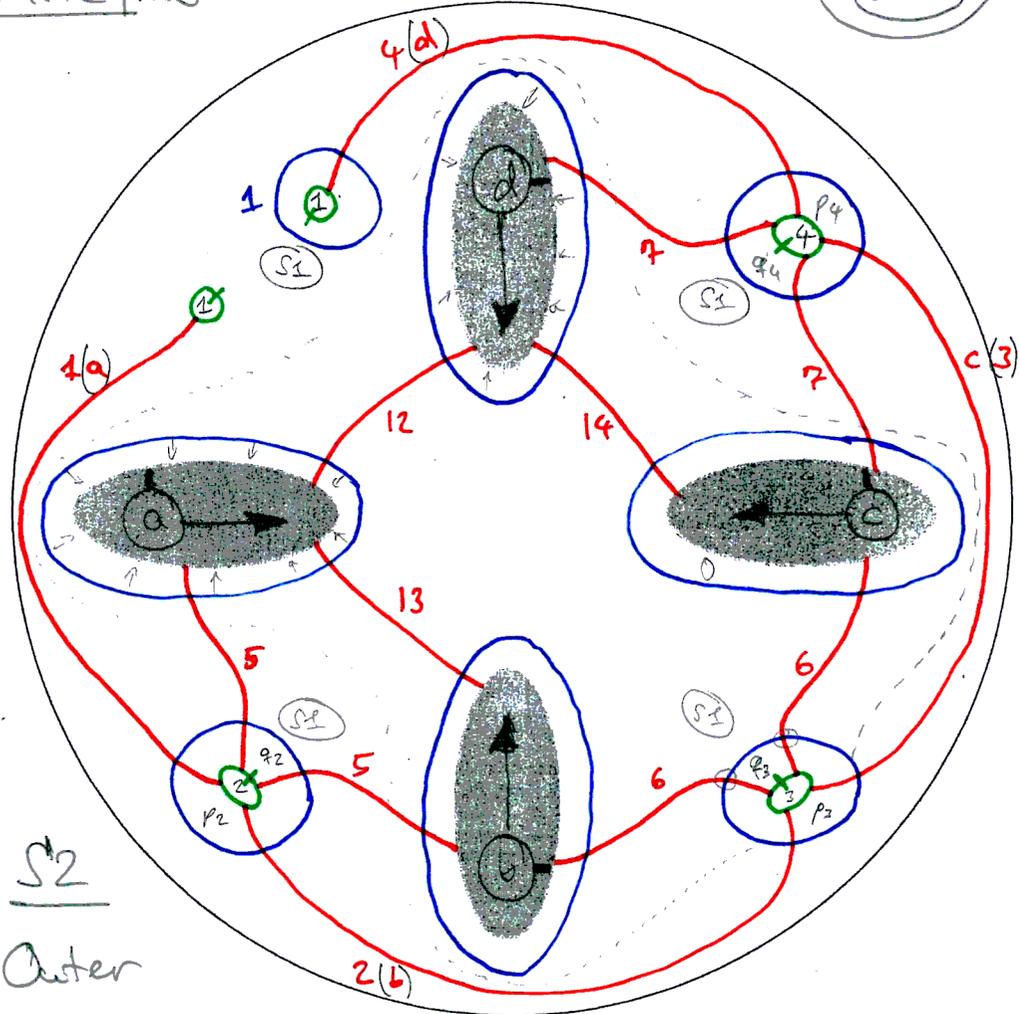

$S_2$

Outer

$S_1$   
 $p_1 = q_1 = 0$

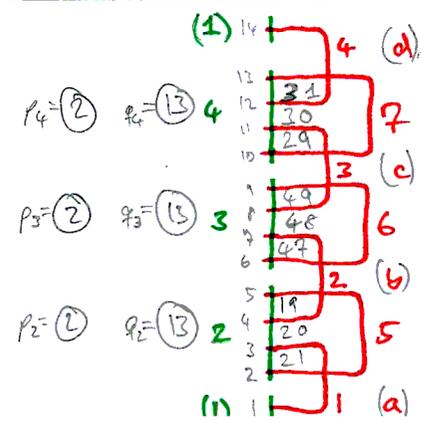

$S_2$   
 $p_3 = q_3 = 0$

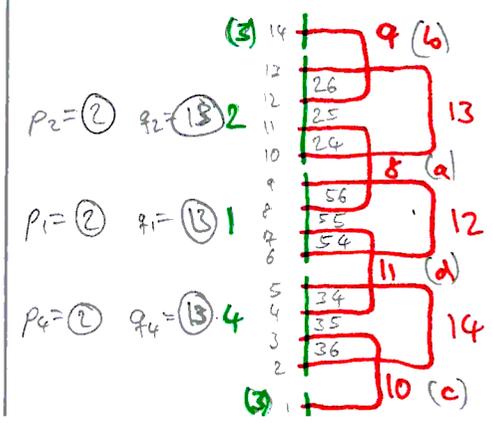

outer  
inner

Back

Gluing BSAAx4e .ub

unified

Front

inner  
outer

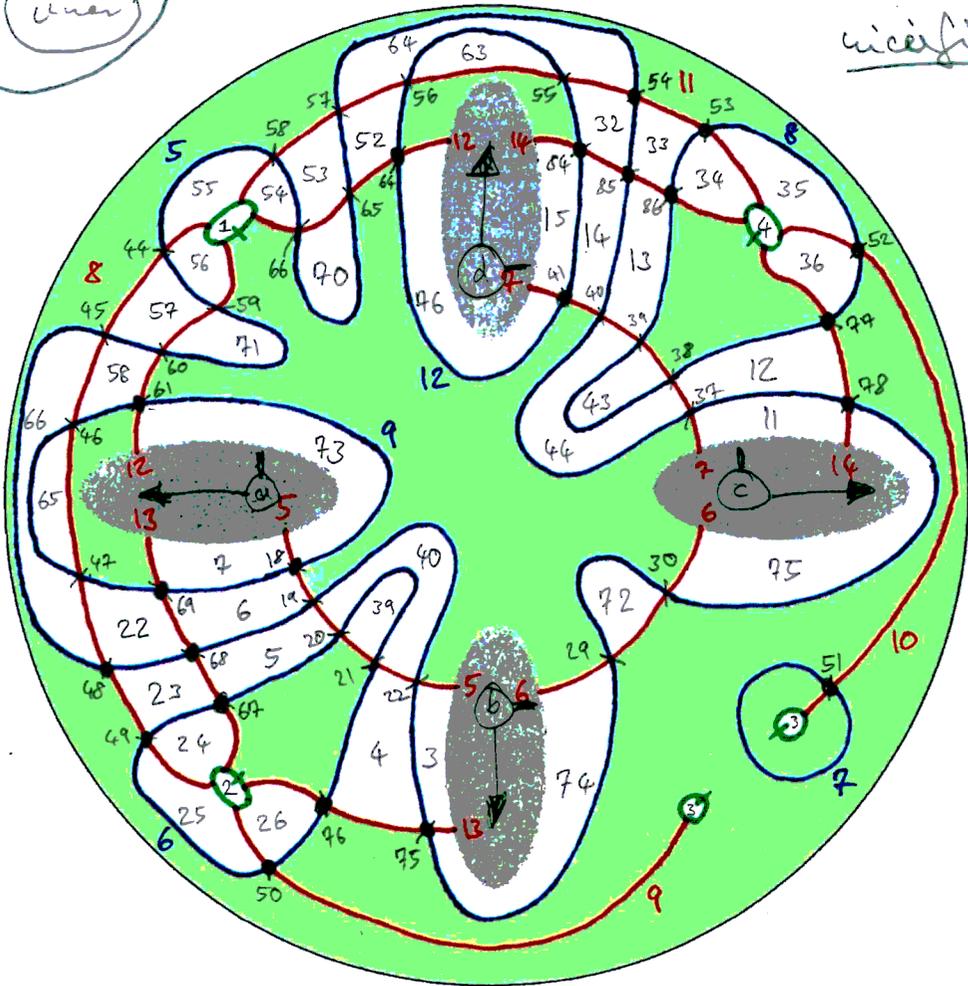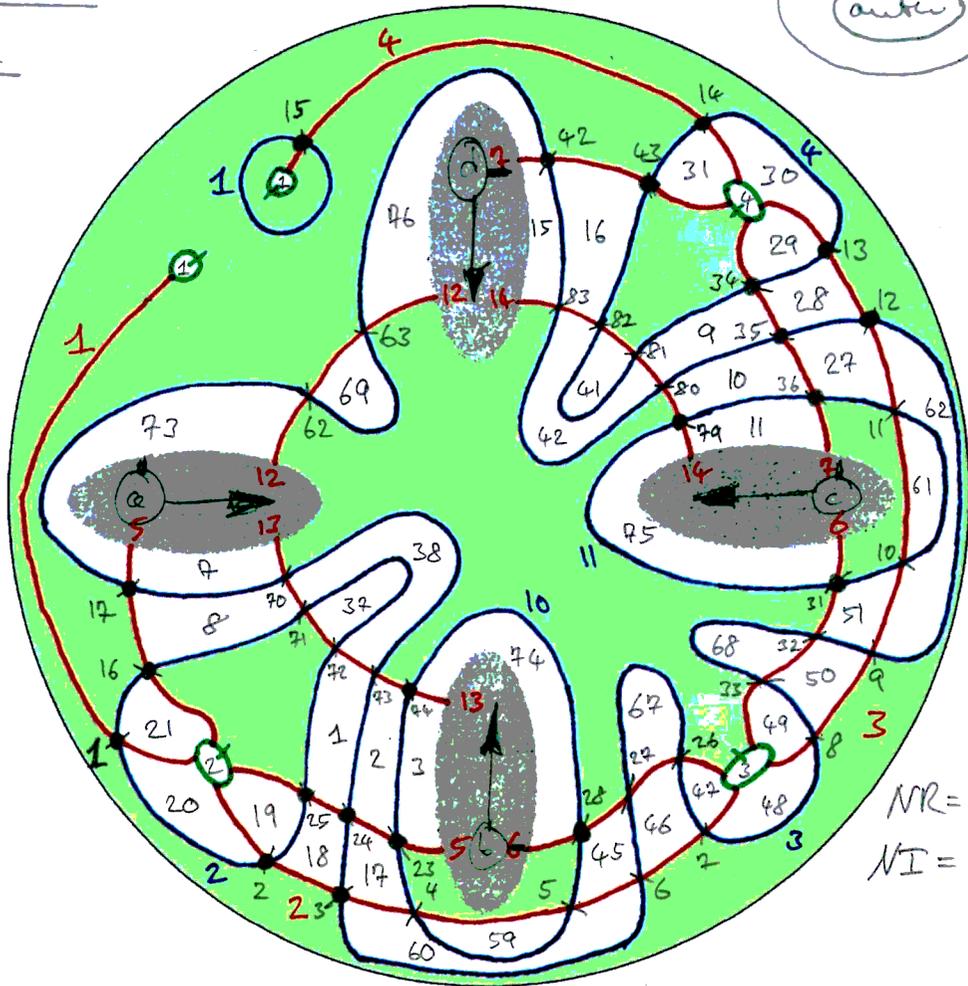

NR=76  
NI=86
